# Supplementary material for: Blind Map Level Systematics Cleaning: A Quadratic Estimator Approach
Source: arXiv:2101.09097 source file (2021-07-10)
Supplement: Supplementary file 1 [file appendix.tex]

\section{\label{app:QE appendix}Perturbed spherical harmonic fields}

We define a the complex Stokes parameters as follows:
\begin{equation}
    {}_{\pm}P(\hat{\mathbf{n}})\equiv(Q\pm iU)(\hat{\mathbf{n}}) = -\sum_{lm}(E_{lm}\pm iB_{lm}) _{\pm2}Y_{lm}(\hat{\mathbf{n}})\;.
\end{equation}
Here we have decomposed the polarization in terms of spin weighted spherical harmonics \cite{2005LNP...653...71C}.
The inverse of this decomposion is then simply written as
\begin{equation}
\begin{gathered}
    E_{lm} \pm iB_{lm} = -\int d\hat{\mathbf{n}}\,(Q\pm iU)(\hat{\mathbf{n}}) _{\pm2}Y^{*}_{lm}\;,\label{Spherical 1}\\
    E^{*}_{lm} \mp iB^{*}_{lm} = -\int d\hat{\mathbf{n}}\,(Q\mp iU)(\hat{\mathbf{n}}) _{\pm2}Y_{lm}\;.\\
\end{gathered}
\end{equation}
The individual expansion coefficients for the $E$ and $B$ polarisation modes can be written as

\begin{gather}\label{elm spin weight}
    E_{lm} = -\frac{1}{2}\int d\hat{\mathbf{n}}\,\left[{}_{+}P(\hat{\mathbf{n}}) _{+2}Y^{*}_{lm}(\hat{\mathbf{n}}) + {}_{-}P(\hat{\mathbf{n}}) _{-2}Y^{*}_{lm}(\hat{\mathbf{n}})\right]\;,\\
    \label{blm spin weight}
    B_{lm} = -\frac{1}{2i}\int d\hat{\mathbf{n}}\left[{}_{+}P(\hat{\mathbf{n}}) _{+2}Y^{*}_{lm}(\hat{\mathbf{n}})-{}_{-}P(\hat{\mathbf{n}}) _{-2}Y^{*}_{lm}(\hat{\mathbf{n}})\right]\;.
\end{gather}

Following the approach seen in \cite{2010PhRvD..81f3512Y}, a perturbative correction to the stokes parameters leads to the following correction to the $E_{lm}$ field:
\begin{equation}
    \delta E_{lm} = -\frac{1}{2}\int d\hat{\mathbf{n}}\left[{}_{+}\delta P(\hat{\mathbf{n}}){}_{+2}Y^{*}_{lm} + {}_{-}\delta P(\hat{\mathbf{n}}){}_{-2}Y^{*}_{lm}\right]\;.
\end{equation}
Inserting the correction to the stokes parameters from \eqref{eqn:Stokes Parameter Perturbation} gives 
\begin{eqnarray}
    \delta E_{lm} =&&\, -\frac{1}{2}\int d\hat{\mathbf{n}}\Bigg[(\gamma^{Q}+i\gamma^{U})(\hat{\mathbf{n}})\Tilde{T}(\hat{\mathbf{n}}){}_{+2}Y^{*}_{lm}\nonumber\\
    &&\,+ (\gamma^{Q}-i\gamma^{U})(\hat{\mathbf{n}})\Tilde{T}(\hat{\mathbf{n}}){}_{-2}Y^{*}_{lm}\Bigg]\;. 
\end{eqnarray}
Expanding in harmonic space gives
\begin{eqnarray}
    \delta E_{lm} =&&\,\frac{1}{2}\sum_{LM}\sum_{l_{2}m_{2}}T_{l_{2}m_{2}}\bigg[(\gamma^{E}_{LM} + i\gamma_{LM}^{B})\nonumber\\
    &&\,\times\int d\hat{\mathbf{n}}{}_{+2}Y_{LM}Y_{l_{2}m_{2}}{}_{+2}Y^{*}_{lm}+
    (\gamma_{LM}^{E} - i\gamma_{LM}^{B})\nonumber\\
    &&\,\times\int d\hat{\mathbf{n}}{}_{-2}Y_{LM}Y_{l_{2}m_{2}}{}_{-2}Y^{*}_{lm}\bigg]\;.
\end{eqnarray}
Using the identity from \citep{Varshalovich:1988ye},
\begin{equation}
\int d\hat{\mathbf{n}}{}_{\pm s}Y_{LM}{}_{0}Y_{l_{2}m_{2}}{}_{\pm s}Y^{*}_{lm} = \xi^{LM}_{lml_{2}m_{2}} \left(\begin{array}{ccc}
         l & L & l_{2}\\
         \mp s & \pm s & 0\\ 
    \end{array}\right)
\end{equation} gives
\begin{eqnarray}
   \delta E_{lm} =&&\, \frac{1}{2}\sum_{LM}\sum_{l_{2}m_{2}}T_{l_{2}m_{2}}\xi^{LM}_{lml_{2}m_{2}}\bigg[(\gamma_{LM}^{E} + i\gamma_{LM}^{B})\nonumber\\ &&\,\times
    \left(\begin{array}{ccc}
         l  & L & l_{2} \\
         -2 & 2 & 0 \\
    \end{array}\right)
    +
    (\gamma_{LM}^{E} - i\gamma_{LM}^{B})\nonumber\\
    &&\,\times
    \left(\begin{array}{ccc}
         l &  L & l_{2} \\
         +2 & -2 & 0 \\ 
    \end{array}\right)\bigg]\;,
\end{eqnarray}
where
\begin{eqnarray}
\xi^{LM}_{lml_{2}m_{2}} =&&\, (-1)^{m}\,\sqrt{\frac{(2l+1)(2L+1)(2l_{2}+1)}{4\pi}}\nonumber\\
&&\,\times\left(\begin{array}{ccc}
         l & L & l_{2}  \\
         -m & M & m_{2} \\ 
    \end{array}\right)    
\end{eqnarray}
Using appropriate identities for the Wigner3j symbols the $\delta E_{lm}$ terms can be re-expressed in form seen in \eqref{eqn:delta elm gamma E} and \eqref{eqn:delta elm gamma B},
\begin{equation}
    \label{delta elm}
    \delta E_{lm} = \sum_{LM}\sum_{l_{2}m_{2}}\gamma_{LM}^{E}T_{l_{2}m_{2}}\xi^{LM}_{lml_{2}m_{2}}\mathcal{H}^{L}_{ll_{2}}\;,
\end{equation}
for $l+L+l_{2} =$ even, and
\begin{equation}
    \delta E_{lm} =
    -i\sum_{LM}\sum_{l_{2}m_{2}}\gamma_{LM}^{B}T_{l_{2}m_{2}}\xi^{LM}_{lml_{2}m_{2}}\mathcal{H}^{L}_{ll_{2}}\;,
\end{equation}
for $l+L+l_{2} =$ odd.
We define $\mathcal{H}^{L}_{ll_{2}}$ as 
\begin{equation}
    \mathcal{H}^{L}_{ll_{2}} = \left(
    \begin{array}{ccc}
         l & L & l_{2}  \\
         2 & -2 & 0 \\
    \end{array}
    \right)\;.
\end{equation}
One can follow a simlilar procedure for the B mode term, starting from equation \eqref{blm spin weight},
\begin{eqnarray}
         \delta B_{lm} =&&\, -\frac{1}{2i}\int d\hat{\mathbf{n}}\left[{}_{+}\delta P(\hat{\mathbf{n}}) _{+2}Y^{*}_{lm}(\hat{\mathbf{n}})-{}_{-}\delta P(\hat{\mathbf{n}}) _{-2}Y^{*}_{lm}(\hat{\mathbf{n}})\right]\;,\nonumber\\
         =&&\, \frac{i}{2}\int d\hat{\mathbf{n}}\Big[(\gamma^{Q}+i\gamma^{U})(\hat{\mathbf{n}})\Tilde{T}(\hat{\mathbf{n}}){}_{+2}Y^{*}_{lm}(\hat{\mathbf{n}})\nonumber\\
         &&\,-(\gamma^{Q}-i\gamma^{U})(\hat{\mathbf{n}})\Tilde{T}(\hat{\mathbf{n}}){}_{-2}Y^{*}_{lm}(\hat{\mathbf{n}})\Big]\;.
\end{eqnarray}
Following on from this, in harmonic space this becomes
\begin{eqnarray}
    \delta B_{lm} =&&\, -\frac{i}{2}\sum_{LM}\sum_{l_{2}m_{2}}T_{l_{2}m_{2}}\bigg[(\gamma^{E}_{LM} + i\gamma_{LM}^{B})\nonumber\\
    &&\,\times\int d\hat{\mathbf{n}}{}_{+2}Y_{LM}Y_{l_{2}m_{2}}{}_{+2}Y^{*}_{lm}-
    (\gamma_{LM}^{E} - i\gamma_{LM}^{B})\nonumber
    \\&&\,\times\int d\hat{\mathbf{n}}{}_{-2}Y_{LM}Y_{l_{2}m_{2}}{}_{-2}Y^{*}_{lm}\bigg]\;.
\end{eqnarray}
We use the procedure used to derive the forms of $\delta E_{lm}$ to show that $\delta B_{lm}$ takes the forms seen in \eqref{eqn:delta blm gamma E} and \eqref{eqn:delta blm gamma B},
\begin{eqnarray}
    \delta B_{lm} = \sum_{LM}\sum_{l_{2}m_{2}}\gamma_{LM}^{B}T_{l_{2}m_{2}}\xi^{LM}_{lml_{2}m_{2}}\mathcal{H}^{L}_{ll_{2}}\;,\;,
\end{eqnarray}
for $l+L+l_{2} =$ even, and
\begin{eqnarray}
    \delta B_{lm} =
    i\sum_{LM}\sum_{l_{2}m_{2}}\gamma_{LM}^{E}T_{l_{2}m_{2}}\xi^{LM}_{lml_{2}m_{2}}\mathcal{H}^{L}_{ll_{2}}\;,
\end{eqnarray}
for $l+L+l_{2} =$ odd.
\section{\label{app:QE appendix 2}$\widehat{J}^{LM}_{lml'm'}$ and $\widehat{K}^{LM}_{lml'm'}$ estimators}
From equations \eqref{eqn:deltaB E cross gamma B} and \eqref{eqn:deltaB E cross gamma E}, and the definitions of $J^{LM,\,XX'}_{lml'm'}$ and $K^{LM,\,XX'}_{lml'm'}$ in section \ref{sec:qe} we note that
\begin{align}
    \left\langle X_{lm}(X'_{l'm'})^{*}\right\rangle =& \sum_{LM}J^{LM,\,XX'}_{ll'}\xi^{LM}_{lml'm'}\;,\\
    \left\langle X_{lm}(X'_{l'm'})^{*}\right\rangle =& \sum_{LM}K^{LM,\,XX'}_{ll'}\xi^{LM}_{lml'm'}\;,
\end{align}
where $\{X,X'\}\in\{T,E,B\}$.
It is possible then to write the estimators $J^{LM,\,XX'}_{ll'}$ and $K^{LM,\,XX'}_{ll'}$ as follows:
\begin{equation}
    \widehat{J}^{LM,\,XX'}_{ll'} = (G^{L}_{ll'})^{-1}\sum_{mm'}X^{\rm map}_{lm}X'^{\,\rm map}_{l'm'}\xi^{LM}_{lml'm'}\;,
\end{equation}
for $l+l'+L =$ even, and
\begin{equation}
    \widehat{K}^{LM,\,XX'}_{ll'} = (G^{L}_{ll'})^{-1}\sum_{mm'}X^{\rm map}_{lm}X'^{\,\rm map}_{l'm'}\xi^{LM}_{lml'm'}\;,
\end{equation}
for $l+l'+L =$ odd.
\par 
Here $C^{ll'}_{AA'}$ is a covariance matrix given as 
\begin{eqnarray}\label{J covariance}
\mathcal{C}^{ll'}_{AA'} \equiv &&\, G^{L}_{ll'}\bigg(\left\langle\widehat{J}^{LM,\,A}_{ll'}\left(\widehat{J}^{LM,\,A'}_{ll'}\right)^{*}\right\rangle\nonumber \\&&\, - \left\langle\widehat{J}^{LM,\,A}_{ll'}\right\rangle\left\langle\widehat{J}^{LM,\,A'}_{ll'}\right\rangle \bigg)\;.
\end{eqnarray}
Consider the specific case of the off diagonal $T$-$B$ correlations. In this case
\begin{gather}
\mathcal{C}^{ll'}_{BTBT} = C^{BB,\,\rm map}_{l}C^{TT\,\rm map}_{l'}\;\nonumber,\\
\mathcal{C}^{ll'}_{TBTB} = C^{TT,\,\rm map}_{l}C^{BB\,\rm map}_{l'}\;\nonumber,\\
\mathcal{C}^{ll'}_{TBBT} = \mathcal{C}^{ll'}_{BTTB} = 0\;.
\end{gather}
